# Supplementary material for: Pion induced double charge exchange reactions in the Delta resonance region
Source: arXiv:nucl-th/0607016 source file (2006-07-10)
Supplement: Supplementary file 1 [file appendix.tex]

%\subsection{Derivation of loss term}
%The aim of this section is to derive the gain and loss terms of the Boltzmann equation in the case of one fermionic particle species scattering via $2\to 2$ processes. In the following the potentials are neglected. Let us formerly write 
%\[
%\frac{df_1(\vec{r},\vec{p}_{A},t)}{dt}
%=\left.  \frac{df_1(\vec{r},\vec{p}_{A},t)}{dt}  \right|_{loss}
%- \left.  \frac{df_1(\vec{r},\vec{p}_{A},t)}{dt}  \right|_{gain}
%\]
%to denote the gain and the loss contribution in the change of the distribution function.
%\subsubsection{Loss term}
We want to evaluate the loss of particle density in the phase space cell $(\vec{r},\vec{p}_A)$ in terms of collisions of particles of momenta $\vec{p_A}$ with particles with momenta $\vec{p}_B$ at position $\vec{r}$. This can be described by the number of collisions per time which is given for all momenta by 
\begin{eqnarray*}
\int \frac{d^3 p_A}{(2\pi)^3} \left. \frac{d\f{A}}{dt}\right|_{loss}=\frac{\mbox{number of reactions $A+B\to a + b$ at } (\vec{r},t)}{\mbox{time $\times$ space-volume}}
&=& \int \sigma(A+B\to a + b) \E_a\E_b d\Phi_{AB}(\vec{r})
\end{eqnarray*}
where $\Phi_{ab}$ is the flux of particles with momenta $\vec{p}_A$ and $\vec{p}_B$ at position $\vec{r}$. The factors $\E_x=(1- f_{1}(\vec{r},\vec{p_{x}},t))$  implement Pauli blocking in the final states. Furthermore,
\[
d\Phi_{AB}(\vec{r})=\f{A} \f{B} v_{AB} \frac{ d^3 p_A }{(2\pi)^3}\frac{d^3p_B}{(2\pi)^3} \; .
\]
So we get 
\begin{eqnarray}
I_{\mathrm{loss}}(\vec{r},\vec{p}_{A},t)
&=&\left. \frac{d\f{A}}{dt}\right|_{loss} 
=\int \sigma(A+B\to a + b)  \E_a\E_b\f{A} \f{B} v_{AB} \  \frac{d^3p_B}{(2\pi)^3} \nonumber \\
&=&\int \frac{d\sigma(A+B\to a + b)}{d\Omega\left(\measuredangle\left[ \vec{p}_{a},\vec{p}_{A}\right]\right)} \E_a\E_b  \f{A} \f{B} v_{AB}   \ d\Omega\left(\measuredangle\left[ \vec{p}_{a},\vec{p}_{A}\right]\right) \frac{d^3p_B}{(2\pi)^3} \; .
\label{lossDeriv}
\end{eqnarray}
